# Supplementary material for: Designing Quaternary Hydrides with Potential High T$_c$ Superconductivity
Source: arXiv:2403.01688 source file (2024-07-23)
Supplement: Supplementary file 1 [file SI_quaternaries.pdf]

# SUPPLEMENTARY INFORMATION

## Designing Quaternary Hydrides with Potential High $T_c$ Superconductivity

Adam Denchfield,<sup>1</sup> Russell J. Hemley,<sup>1,2,3</sup> and Hyowon Park<sup>1,4</sup>

<sup>1</sup>*Department of Physics, University of Illinois Chicago, Chicago, Illinois 60607, USA*

<sup>2</sup>*Department of Chemistry, University of Illinois Chicago, Chicago, Illinois 60607, USA*

<sup>3</sup>*Department of Earth and Environmental Sciences,*

*University of Illinois Chicago, Chicago, Illinois 60607, USA*

<sup>4</sup>*Materials Science Division, Argonne National Laboratory, Lemont, Illinois 60439, USA*

(Dated: July 1st, 2024)

### More on $\text{Lu}_4\text{H}_{11}\text{O}$

The phonon dispersion and superconducting properties are further elucidated in Fig. 1. We show the Fermi surface of  $\text{Lu}_4\text{H}_{11}\text{O}$  at 25 GPa [Fig. 1(b)]. The phonon-averaged electron-phonon coupling  $\lambda_{nk}$  and superconducting gap  $\Delta_{nk}$  at 50 K are projected on the Fermi Surface and illustrate a band-dependent s-wave gap structure [Fig. 1(c,d)], with the surface discretization reflecting the underlying mesh. Additional Fermi sheets shown correspond to bands 3 eV below  $E_F$  which EPW unexpectedly predicts contribute to the electron-phonon coupling. The phonon dispersion illustrates the strongest EPC is from a few  $q \neq 0$  modes, and  $\lambda_{nk}$  illustrates the strongest EPC on the FS is near the  $X$ -pt, likely reflecting the nearby van Hove singularity 0.36 eV below  $E_F$  at  $k = X$ . We note that the electron-phonon coupling increases if  $E_F$  is reduced by 0.36 eV, coupled with an increase in the size of the strongly-coupled Fermi sheet, which increases  $T_c$  slightly to 140 K and induces a multigap structure like  $\text{LaH}_{10}$  [1].

### More on $(\text{CaH}_{11})_2 \text{Sc}_6\text{NH}$

As displayed in Figure 5 in the main text, the dynamical matrix at  $q = 0$  of the  $(\text{CaH}_{11})_2 \text{Sc}_6\text{NH}$  conventional cell at 20 GPa has three eigenvectors with imaginary frequencies. The energy gained from the distortions associated with the mode with largest imaginary frequency is 7 meV/hydrogen at this pressure, which makes it unclear if nuclear quantum effects and thermal effects would stabilize the high symmetry structure. Lowering the pressure deepens the double well, as well as introduces more phonon modes with imaginary frequencies. Raising pressure reduces the energy gain from such distortions, but it is worth finding if the distortions would interfere with superconductivity in the first place.

Therefore we investigate the electronic properties of the classically distorted structure at the minimum of the PES for the eigenmode with largest imaginary frequency. We find that the hydrogen DOS has not changed much (consistent with the low energy gain from distortion; see Fig. S12), yet the hydrogen displacements massively improve the hydrogen sublattice connectivity (as measured by  $\phi_{iso}^{net}$  from the ELF), with  $\text{H}^{oct}\text{-H}^{tet}$  distances decreasing

from 2 Å to 1.74 Å (Fig. 3). This gives rise to a large increase of the  $\phi_{iso}^{net} = 0.695$  and therefore  $T_c^{net}$  rises to 220 K. It is possible that this symmetry-breaking of the octahedral hydrogen enhancing  $T_c$  is a more general phenomenon, and may in fact responsible for the high  $T_c$  reported in N-doped  $\text{LuH}_3$  [2]. Such H-H distances have recently been observed in other metal hydrides [3, 4].

Other choices of Y,Z on the electronic properties of  $(\text{CaH}_{11})_2\text{Sc}_6\text{YZ}$  can also enhance  $T_c^{net}$ . We show the electronic structure at ambient conditions of a few permutations in Figure S15. At ambient pressures it appears  $T_c^{net}$  is highest at 182 K with Y=N and Z being unoccupied (i.e.  $\text{Sc}_{0.75}\text{Ca}_{0.25}\text{H}_{2.75}\text{N}_{0.125}$ ).

### DOS Trends & DFT+U Dependence

A trend can be seen for some of the compositions seen in Figures 9 and 18. There is a common shape to the DOS near  $E_F$ , highlighted for four examples in Fig. 17. This is encouraging, as it illustrates the chemistry is similar among different compositions. In particular, this electronic structure is associated with the quantum interference caused by the Lewis base (N,O,S,P), as shown in our work on  $\text{Lu}_8\text{H}_{23}\text{N}$  [5].

Out of the examples shown, we found only significant dependence on U (on the rare earth d-orbitals) for the cases involving rare earth nitride/oxide units. This is expected, as for example the rare earth nitrides' semiconducting properties severely change with U using PBE with PAW pseudopotentials [6], going from a bandgap of  $\sim 0.1$  eV to  $\sim 1$  eV (the latter being the experimental bandgap). We leave a more thorough investigation of correlation effects for future work.

### Counterexamples where $\text{DOS}_H(E_F)$ isn't dominant

It is important to understand that the model structures discussed in the main text do not guarantee a hydrogen-dominant  $\text{DOS}(E_F)$ , and that some care must be taken in choosing the components. We show three such poor choices for the second model structure (all with R=Lu) in Fig. 8. The first example using X=Sr, Y=N, Z=H (left) only has a weakly dominant hydrogen DOS, and the minimum in the  $\text{DOS}(E_F)$  implies a lower  $T_c$ . The DOS max-

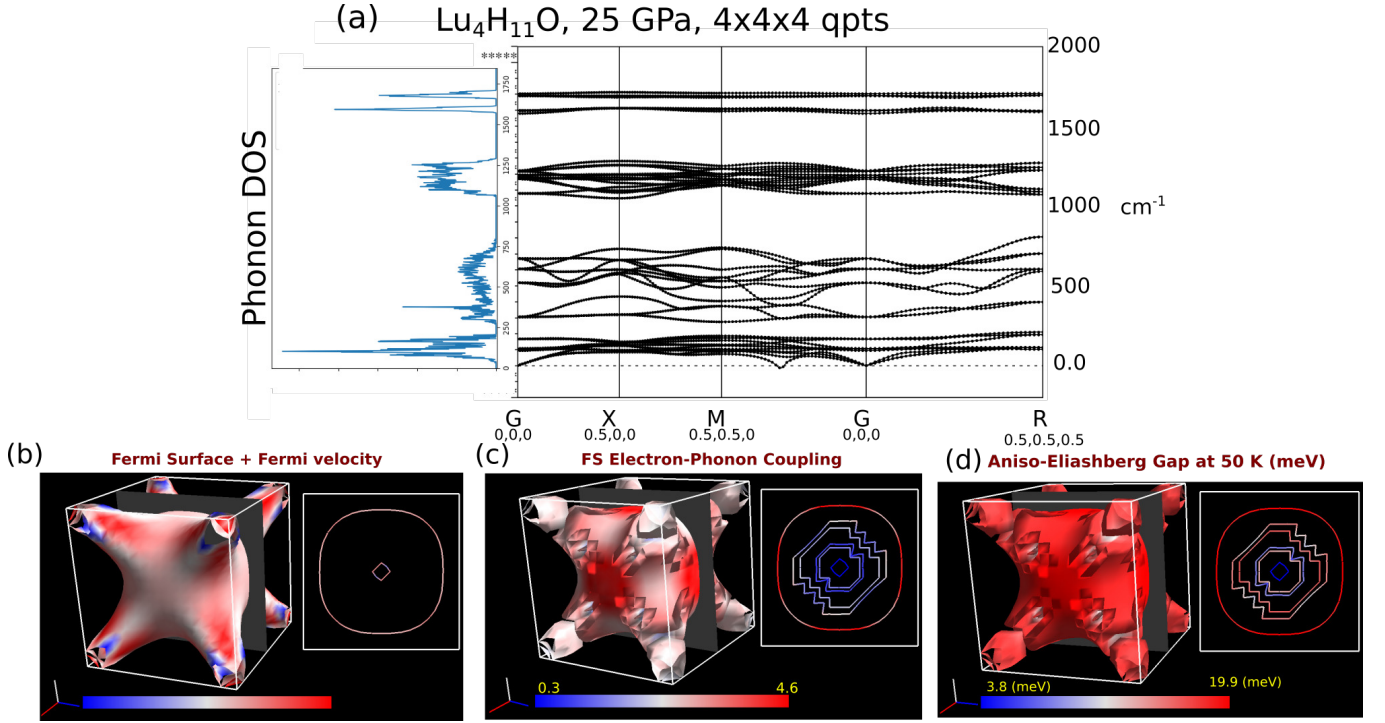

FIG. 1: Vibrational and superconducting properties of  $\text{Lu}_4\text{H}_{11}\text{O}$  at 25 GPa. (a) The phonon dispersion and density of states, (b) electronic Fermi surface for reference, (c) FS-projected electron-phonon coupling, and (d) FS-projected superconducting gap at 50 K. The additional Fermi sheets in (c) and (d) not present in (b) are bands present 2.5 eV below  $E_F$ , which is automatically added to the EPW output of these quantities.

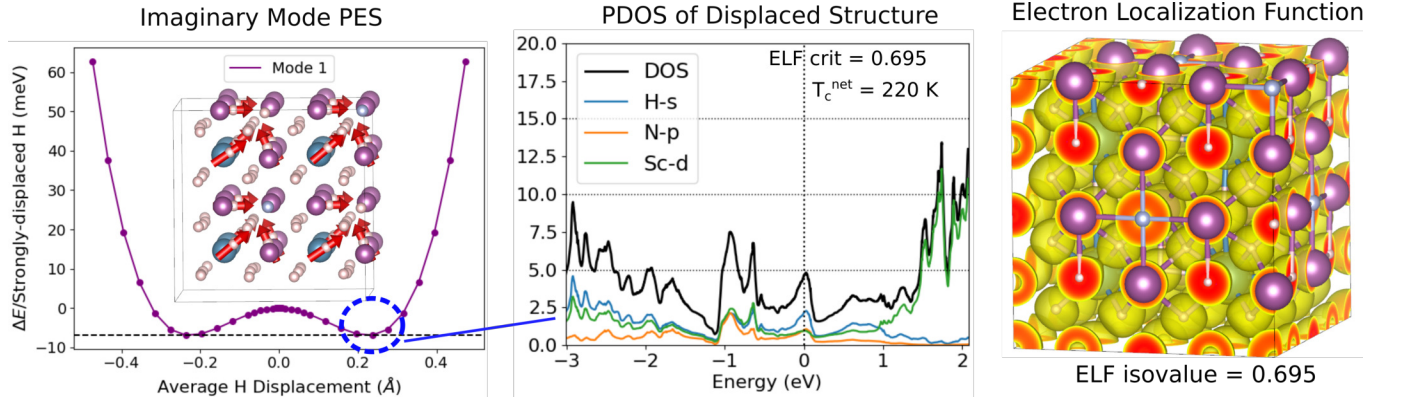

FIG. 2: Electronic and vibrational properties of  $\text{Sc}_6\text{Ca}_2\text{H}_{23}\text{N}$  at 20 GPa at the potential energy surface (PES) minimum with respect to the perturbation shown.

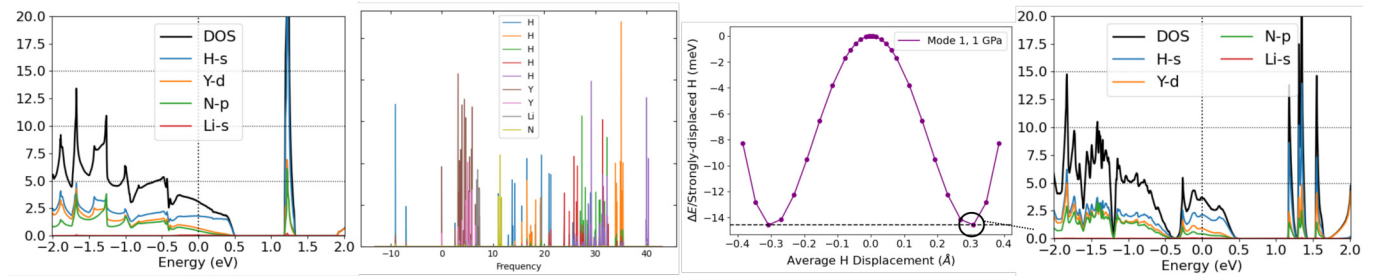

FIG. 3: Electronic and vibrational properties of  $\text{Y}_7\text{LiH}_{22}\text{N}$  at 1 GPa at the potential energy surface (PES) center (left) and minimum (right) with respect to displacing hydrogen along the mode with largest imaginary frequency. Increasing pressure weakens the double well anharmonicity.

ima are above  $E_F$ ; typically we find one can resolve this doping problem by pairing atoms corresponding to ionic insulators (i.e. II-VI, III-VI, rare earth nitrides, etc). In fact, insulating units for choices of X,Y tends to make the auxiliary cage inert. For example, the X=Ti,Y=Z=C example (middle) features a Ti-d dominated DOS( $E_F$ ) because the carbon does not gap the Ti; in fact TiC is not insulating. In the last example, we used a cubic semiconductor YbO to choose X=Yb, Y=O,Z=H. However, the unfilled f-shell in Yb participates at  $E_F$ . This can be understood as the YbO bandgap for thin films is only 0.25 eV [7], making it likely that the H/Lu environment hybridizes with the YbO units to eliminate the bandgap. Generally it appears wise to avoid compounds with unfilled f-shells. These counterexamples help inform us that only charge transfer or hole-doping alone does not yield the desired electronic structure.

### Model Structure $(\text{RH}_{11})_2\text{X}_6\text{YZ}$ Inversion

We compute the effect of ‘inverting’ the structural motif of an  $\text{RH}_{11}$  unit protected by an  $\text{X}_6\text{YZ}$  cage in the  $(\text{RH}_{11})_2\text{X}_3\text{YZ}$  structure in the main text by swapping the roles of the R and X atoms, visualized in Fig. 21. The PDOS of  $(\text{CaH}_{11})_2(\text{Y}_6\text{OH})$  looks like an electron-doped version of  $(\text{YH}_{11})_2(\text{Ca}_6\text{OH})$  despite the fact that the oxygen atoms are now near Y instead of Ca. Charge transfer from yttrium to oxygen now occurs, and while YO is not known to be insulating, several (Y,H,O) compounds are insulating. However, we note the ELF hydrogen networking isovalue  $\phi_{iso}^{net}$  decreases from 0.53 to 0.49 upon this swap, which lowers the estimated  $T_c$  by  $\approx 50$  K.

### Stability

We believe the best choices stability-wise for the cubic structure involve using well-known cubic semiconducting/insulating combinations where X also forms cubic alloys with R, such as  $\text{RXY} = \text{YCaO/ScAlN}$ . As an illustrative counterexample, if we choose  $\text{R}=\text{Lu}$  and  $\text{X}=\text{Na}$ , the two are not known to form a cubic alloy, even though the Lu, Na radii are similar. We indeed find  $\text{RXYZ} = \text{LuNaH}_2$  using the above structure is not even metastable. However, we have found doping some examples such as  $(\text{ScH}_{11})_2$  ( $\text{Mg}_4\text{Li}_2\text{NH}$ ) results in hydrogen-dominant states at  $E_F$  with only a moderate tetragonal distortion away from cubic.

We note that quaternary hydride structures based on dense sphere packings were studied in Ref. [8], which have FCC-like packings of the large metal atoms but the locations of the hydrogen atoms differ from the structure presented in this work. Their  $\text{ScY}_2\text{CaH}_{12}$  example had a hydrogen-dominant DOS and was found to be dynamically stable at ambient conditions with a computed  $T_c$  of 5.7 K. This low  $T_c$  despite the large hydrogen DOS is attributed to the large lattice constant and small electron-phonon coupling. Its enthalpy was found to be 78.6 meV/atom higher than that of the decomposition into  $\text{ScH}_3$ ,  $2\text{YH}_3$ ,  $\text{CaH}_2$ , and  $0.5\text{H}_2$ . Considering the computed  $T_c$  of FCC  $\text{LuH}_3$  is much higher at  $\approx 30$  K despite a much lower DOS [9–11], we can infer the electron-phonon coupling associated with the hydrogen configuration in FCC  $\text{RH}_3$  ( $\text{R}=\text{Sc,Y,La,Lu}$ ) is large, which in large part motivates the usage of FCC  $\text{RH}_3$  as a parent structure.

*a. Caveat - Hydrogen Stability* Our results in Figs. 5 and 6 imply that below a critical pressure, the hydrogen sublattices may suffer classical distortions from the high-symmetry structures presented. However, classical DFT-level calculations overestimate the pressure needed to stabilize the hydrogen sublattice in doped  $\text{RH}_3$ , as shown in our work on  $\text{LuH}_{2.875}\text{N}_{0.125}$  [5] where nuclear quantum effects stabilize the structure at 2 GPa despite classical DFT calculations predicting a pressure of 17 GPa for such stabilization.

Hole doping the rare earth in  $\text{RH}_3$  typically leads to hydrogen escaping the material in ambient conditions [12–14]. In DFT-level relaxations this would be reflected by the formation of  $\text{H}_2$  molecules in the unit cell. We find this instability to occur for the  $\text{LuNa}_3\text{H}_{12}$  case considered in Fig. 6(b) even when starting from the high-symmetry initial structure. If we perturb the initial structure away from its high-symmetry starting point, many  $(\text{RH}_{11})_2(\text{X}_6\text{YZ})$  examples also appear to suffer this instability; however, the metastability of such phases can be inferred by the DFT-computed potential energy surface (PES) of the nuclei. For many weakly anharmonic PES, quantum and thermal effects can metastabilize such structures. Computational tools such as the SSCHA [15] have confirmed this to occur for  $(\text{LuH}_{11})_2(\text{Lu}_6\text{NH})$  [5] which we confirm suffers the same DFT-level instabil-

TABLE I: Table of selected reference materials for which to compare thermodynamic stability of certain complex hydrides.

| Material                                          | Energy/atom (Ry) [Ambient] | Decomposition                                                                                                                       | $\Delta E$ (eV/atom) |
|---------------------------------------------------|----------------------------|-------------------------------------------------------------------------------------------------------------------------------------|----------------------|
| H <sub>2</sub>                                    | -1.167                     |                                                                                                                                     |                      |
| H <sub>2</sub> O                                  | -14.696                    |                                                                                                                                     |                      |
| LiH                                               | -8.136                     |                                                                                                                                     |                      |
| MgH <sub>2</sub>                                  | -11.997                    |                                                                                                                                     |                      |
| CaH <sub>2</sub>                                  | -25.794                    |                                                                                                                                     |                      |
| ScH <sub>2</sub>                                  | -53.148                    |                                                                                                                                     |                      |
| YH <sub>3</sub>                                   | -22.795                    |                                                                                                                                     |                      |
| LuH <sub>2</sub>                                  | -360.881                   |                                                                                                                                     |                      |
| LuH <sub>3</sub>                                  | -270.894                   |                                                                                                                                     |                      |
| YN                                                | -57.987                    |                                                                                                                                     |                      |
| ScN                                               | -92.732                    |                                                                                                                                     |                      |
| Lu <sub>4</sub> H <sub>11</sub> O                 | -273.484                   | (LuH <sub>3</sub> ) <sub>1</sub> + (LuH <sub>2</sub> ) <sub>3</sub> + (H <sub>2</sub> O) <sub>1</sub>                               | -0.128               |
| Y <sub>7</sub> LiH <sub>23</sub> N                | -21.361                    | (YN) <sub>1</sub> + (LiH) <sub>1</sub> + (YH <sub>3</sub> ) <sub>6</sub> + (H <sub>2</sub> ) <sub>2</sub>                           | 0.188                |
| Y <sub>7</sub> LiH <sub>22</sub> N                | -22.016                    | (1/2) ((YN) <sub>1</sub> + (LiH) <sub>1</sub> + (YH <sub>3</sub> ) <sub>6</sub> + (H <sub>2</sub> ) <sub>3</sub> )                  | 0.141                |
| Sc <sub>6</sub> Mg <sub>2</sub> H <sub>23</sub> N | -33.269                    | (1/2) ((ScN) <sub>2</sub> + (MgH <sub>2</sub> ) <sub>4</sub> + (ScH <sub>2</sub> ) <sub>10</sub> + (H <sub>2</sub> ) <sub>9</sub> ) | 0.238                |
| Sc <sub>6</sub> Ca <sub>2</sub> H <sub>23</sub> N | -35.815                    | (1/2) ((ScN) <sub>2</sub> + (MgH <sub>2</sub> ) <sub>4</sub> + (ScH <sub>2</sub> ) <sub>10</sub> + (H <sub>2</sub> ) <sub>9</sub> ) | 0.795                |
| Sc <sub>7</sub> MgH <sub>23</sub> N               | -37.131                    | (1/2) ((ScN) <sub>2</sub> + (MgH <sub>2</sub> ) <sub>2</sub> + (ScH <sub>2</sub> ) <sub>12</sub> + (H <sub>2</sub> ) <sub>9</sub> ) | 0.183                |

For reference, diamond (Fd $\bar{3}$ m carbon) is 0.136 eV/atom above the convex hull.

ity towards H<sub>2</sub> molecule formation when perturbed away from the high-symmetry structure. Pressure can also stabilize the non-stoichiometric hydrogen fraction. We note Fm3m MgH<sub>3</sub> is stabilized at 100 GPa of pressure [16].

Charged defects (which the X,Y,Z atoms in our model structures can play the role of) may support adsorbed hydrogen [17, 18], but it is unclear if this would meaningfully increase the hydrogen storage capacity in bulk (RH<sub>11</sub>)<sub>2</sub>(X<sub>6</sub>YZ) or the other model structures. Zero-point effects can be quite important for such calculations [19].

#### Harmonic Phonons of Two Examples

In this section we discuss the two examples in Fig. 9 with high predicted  $T_c^{net}$ , ([La/Sc]H<sub>11</sub>)<sub>2</sub>(Mg<sub>6</sub>OH). The most relevant question for applications concerns whether or not these structures are dynamically stable at ambient or near-ambient pressures. While DFT does not account for temperature or quantum nuclear effects (which are large for hydrogen), it is still the most computationally feasible method for studying the vibrational properties of such a large cell. We use the **phonopy**[20] package to compute the harmonic phonons at  $\Gamma$  using the finite displacement method and plot the resulting phonon density of states.

In both cases studied in Fig. 10 there are predominantly hydrogen based modes that indicate instabilities (imaginary frequencies). We find the PBEsol functional for the phonon calculations does not change the results.

#### Anharmonicity Analysis

Despite the instabilities predicted by the harmonic phonon analysis above, it is possible that quantum zero point motion of the hydrogen atoms can stabilize the high-symmetry structure. This has been verified for some hydrides using the SSCHA method [21, 22]. In order to investigate this possibility, we perform a collective-mode reaction-coordinate analysis of the most unstable modes (largest imaginary part) of ([La/Sc]H<sub>11</sub>)<sub>2</sub>(Mg<sub>6</sub>OH). In a related work on Fm3m Lu<sub>8</sub>H<sub>23</sub>N [5], this same analysis showed the instability to be very weak, which we argued would be easily stabilized by quantum zero point motion effects.

The results for ([La/Sc]H<sub>11</sub>)<sub>2</sub>(Mg<sub>6</sub>OH) are shown in Fig. 10, where the FWHM is displayed for hydrogen displacements from SSCHA data on Fm3m Lu<sub>8</sub>H<sub>23</sub>N, indicating the size of quantum zero point motion for a typical hydrogen atom in that system. The energy saved along the reaction coordinates is much larger than that in Lu<sub>8</sub>H<sub>23</sub>N, and amplitude of the energy minimum is also much larger. The biggest differences in the La/Sc cases are that more of the hydrogen atoms contribute to DOS( $E_F$ ) and that some octahedral hydrogen states end up with < 1 electron on average, likely due to the hole-doping effect of X=Mg. It is possible that electron-doping these examples would weaken these anharmonicities. The instabilities are weakened under pressure but do not completely disappear.

If we begin a relaxation from the minima outlined in Fig. 10, the hydrogen appear to disassociate from their positions and form H<sub>2</sub> molecules. Since LaMg<sub>3</sub> is experimentally known to typically only hydrogenate up to

LaMg<sub>3</sub>H<sub>9</sub>[14], it is possible a configuration with a higher R:Mg ratio is needed to sustain the high hydrogen density at ambient pressures.

### Doping

While the parent structures/composition discussed in the main text are fairly flexible, our list of examples in Fig. 9 motivates a desire to account for doping due to the preponderance of large DOS peaks close to  $E_F$ . Electron/hole doping would be useful to tune  $E_F$  closer to a peak to maximize  $T_c$ , and isovalent doping with atoms of different sizes (i.e. La  $\rightarrow$  Sc) can help tune stability of the metal lattice and lattice constant, which can indirectly affect the electronic structure. For example, we note that the primary difference between  $(LaH_{11})_2(Mg_6OH)$  and  $([Y/Sc]H_{11})_2(Mg_6OH)$  is the lattice constant. The shrinking of the lattice constant of  $(LaH_{11})_2(Mg_6OH)$  leads to nearly-isolated hydrogen states more easily forming a metallic network, whose hybridization increases the hydrogen bandwidth, leading to the lower hydrogen DOS( $E_F$ ) in the R=Sc,Y cases.

We therefore generalize the second model structure's chemical formula to include doping of the various parts of the formula:

$$\text{Doped Formula} = (R_{1-x}R'_xH_{11})_2(X_{6-n}X'_nY_{1-\gamma}Y'_\gamma Z_{1-\delta}Z'_\delta)$$

The elements with a tick mark indicate the dopants, which are to be put in the same location as the parent atom.

Let us present an example of using such a formula. Going back to our  $(YH_{11})_2(Mg_6OH)$  example. If we wish to tune the lattice constant and hydrogen distances, we can go about this in various ways:

- Replace some O with S ( $Y' = S$ ), increasing the lattice constant of the  $Mg_6O$  units on average.
- Replace some Mg with Ca ( $X' = Ca$ ), increasing the overall lattice constant of the entire system more uniformly on average and increasing the thermodynamic stability of hydrogen in the system.
- Replace some Y with La ( $R' = La$ ), increasing the size of the  $RH_{11}$  units on average.

On the other hand, if we wanted to electron-dope  $(YH_{11})_2(Mg_6OH)$  to tune  $E_F$  to approach the DOS peak 0.2 eV above  $E_F$ , we could accomplish this in multiple ways, with various pros and cons:

- Replace some O with H ( $Y' = H$ ). The cons are that oxygen presence is vital to the tetrahedral hydrogen states at  $E_F$ , and that this may decrease the thermodynamic stability of the system since  $MgH_3$  is thermodynamically unstable.
- Replace some Mg with Y/Sc ( $Y' = Y/Sc$ ), leading to more electrons in the system. The cons are that

this may lead to a distortion of the cubic cell, which may interfere with the metallic hydrogen sublattice chemistry.

- Replace some Y with Zr/Ce, which both may help electron-dope the system but risks weakening the superconductivity associated with the  $RH_{11}$  units.
- Replace some N/P with O/S in any systems using N/P.

If we wanted to hole-dope any of the above systems, we could go about it multiple ways:

- Replace some octahedral H with O/N/S/P ( $Z' = O/N/S/P$ ). This risks forming O/N/S/P metal states which would interfere with the quantum interference phenomena raising DOS<sub>H</sub>( $E_F$ ).
- Replace some R with a normally 2+ oxidation state element (e.g.  $R' = Mg/Ca/Sr$ ). This risks reducing the number of superconducting  $RH_{11}$  units.
- Replace some O/S with N/P in any systems using O/S.

Many of the electron/hole-doping examples listed above have cons, but should accomplish the desired doping without severely changing the electronic and stability properties if done in small quantities. An example of this is shown in Fig. 18 where we show how the electronic structure of  $YH_{11})_2(Ca_6OH)$  remains unchanged aside from tuning  $E_F$  when electron doping with a pure electron (a), an additional Yttrium atom (b), or hole doping by replacing one of the 4b hydrogen with O. A larger amount of electron doping is necessary to tune  $E_F$  to the flat band in  $(LaH_{11})_2(Sr_6SH)$  at 0.7 eV above  $E_F$ , requiring four extra electrons. This result suggests that one should try simulating  $(LaH_{11})_2(Sr_2La_4SH)$  (choosing  $X' = La, n=4$ ). As one can see, there are many tuning parameters in optimizing the electronic and structural properties for the best superconducting  $T_c$  and ideal stability properties. We leave more analyses of doping effects for future work.

### Additional Methods Details

We performed DFT calculations primarily with the Quantum Espresso software package [23]. The SSSP database [24] was used to vet pseudopotentials for convergence of the computed pressure, phonon frequencies, and formation energies. Accordingly, we chose rare earth pseudopotentials from Ref. [6], and the `pslibrary` pseudopotentials for most other elements [25]. We relaxed systems from the starting model structures defined in the main text using DFT-PBE which generally maintained high symmetry due to the symmetric starting point. Each relaxed structure had remaining forces under  $1e-5$  Ry/Bohr, and energy differences were under  $1e-5$  Ry. We did not relax structures again for the DFT+U

calculations, as DFT+U typically worsens lattice parameter agreement when it corrects for electronic structure [26].

We used wavefunction plane-wave cutoffs of 90-100 Ry for the structures and charge density cutoffs of 360-400 Ry. We generally used tight k-meshes corresponding to  $0.13 \text{ \AA}^{-1}$ , but did convergence tests with more k-points as needed. We also used the optimized tetrahedron method [27] to evaluate the DOS. The **VESTA** code [28] was used for the visualizations of the ELF and ILDOS. ILDOS calculations performed integrations within a range of 5meV around  $E_F$ . We used **Quantum Espresso**'s default atomic projections for the PDOS calculations. We also performed comparisons of the PBE functional with the vdW-DF3-opt2 functional [29] for some of the calculations and saw no meaningful changes.

We performed DFT+U calculations with the U-values recommended in Ref. [25], which vetted the pseudopotentials and U-values with calculations on rare earth nitrides using the same codes and functional we use. We confirmed independently U-values for YN and ScN to match indirect band gaps. The ideal U-value is not tied to the atom, and in principle it should be structure-dependent. Nevertheless, we use a fixed U-value as it is generally difficult to find the ideal U-value for each structure, but U-dependence of the results are investigated. Ref. [6] also recommends  $U=5.5 \text{ eV}$  for  $\text{Lu}_f$  electrons but use of this value did not significantly change the electronic properties near  $E_F$ .

Because we are using the networking-value  $T_c$  estimator[30], we perform DFT calculations using **Quantum Espresso** [23] at the PBE level[31] to match the calculations used to create the networking-value  $T_c$  estimator, as using other functionals would invalidate the usage of the estimator. We use the  $\phi_{iso}^{net}$  computed for  $nspin=1$ ,  $U=0$  as those are the parameters used to establish the estimator [30]

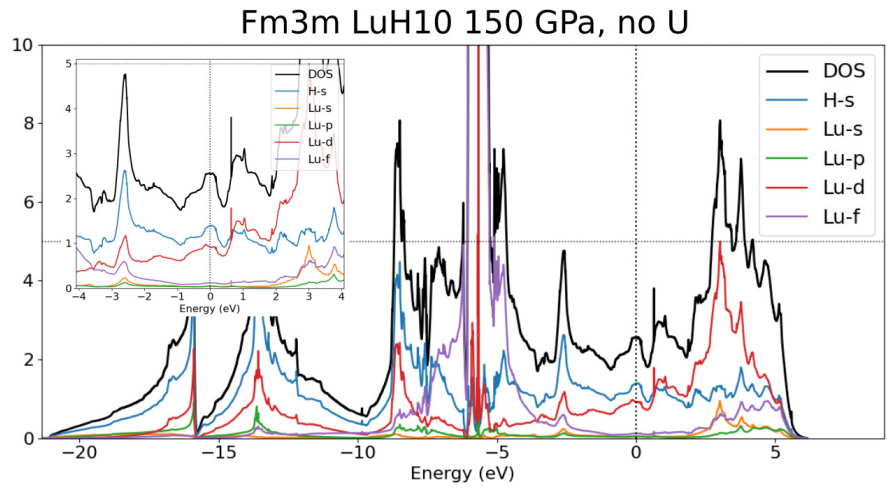

FIG. 4: Computed PDOS of Fm3m LuH<sub>10</sub> at 150 GPa.

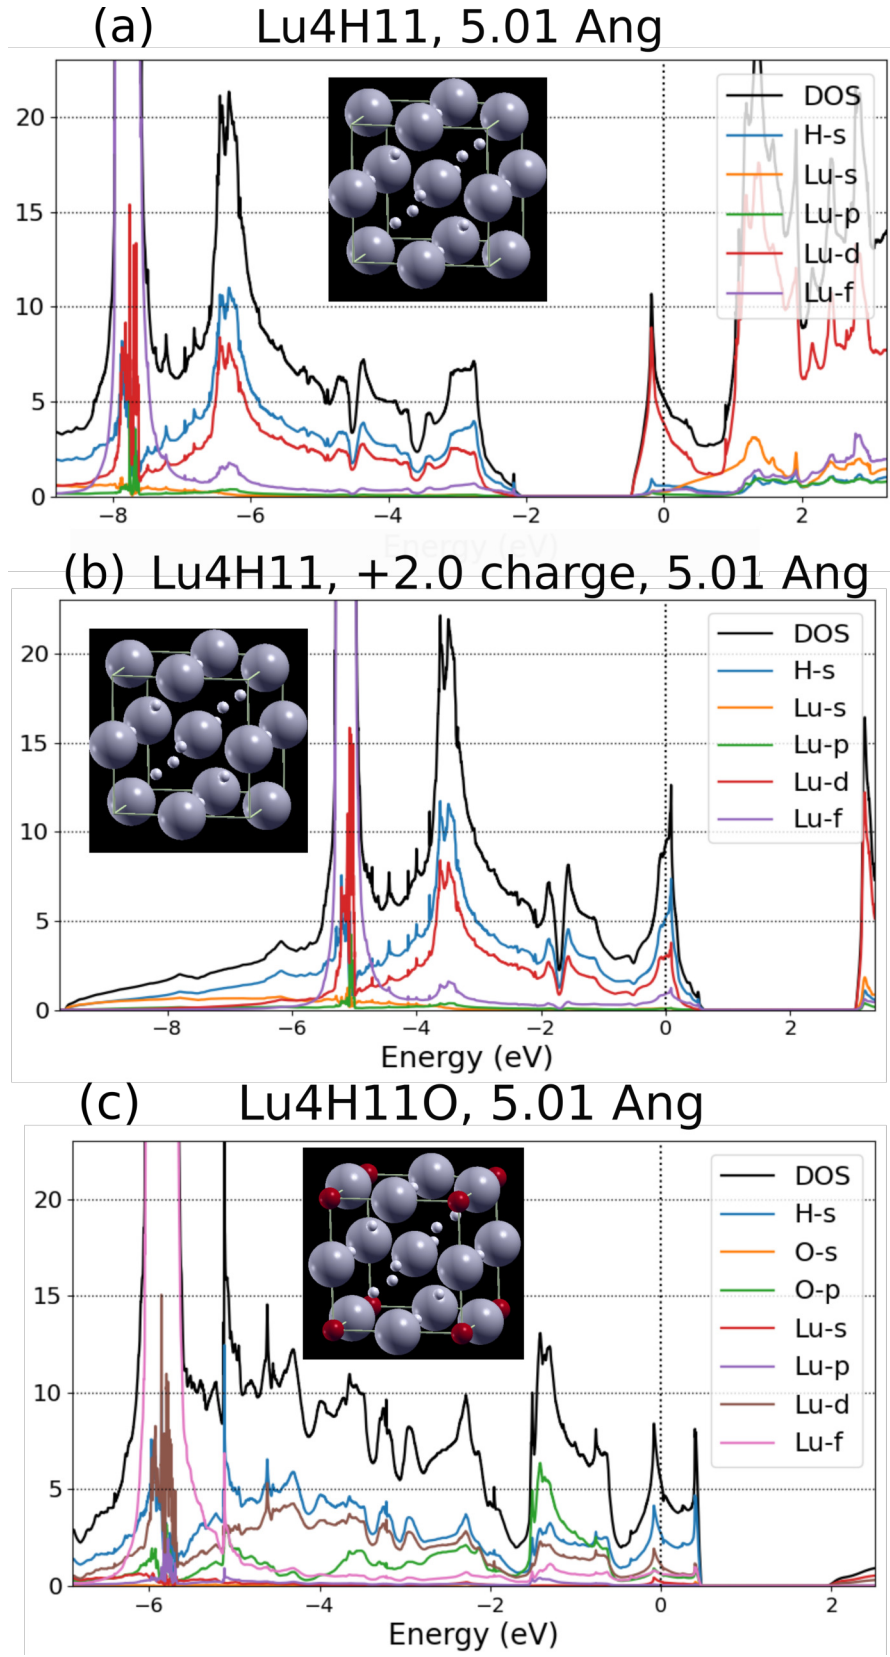

FIG. 5: PDOS with  $U=7.5$  eV of  $\text{Pm}3\text{m}$   $\text{Lu}_4\text{H}_{11}$  (a),  $\text{Lu}_4\text{H}_{11}-2+$  (b), and  $\text{Lu}_4\text{H}_{11}\text{O}$  (c).

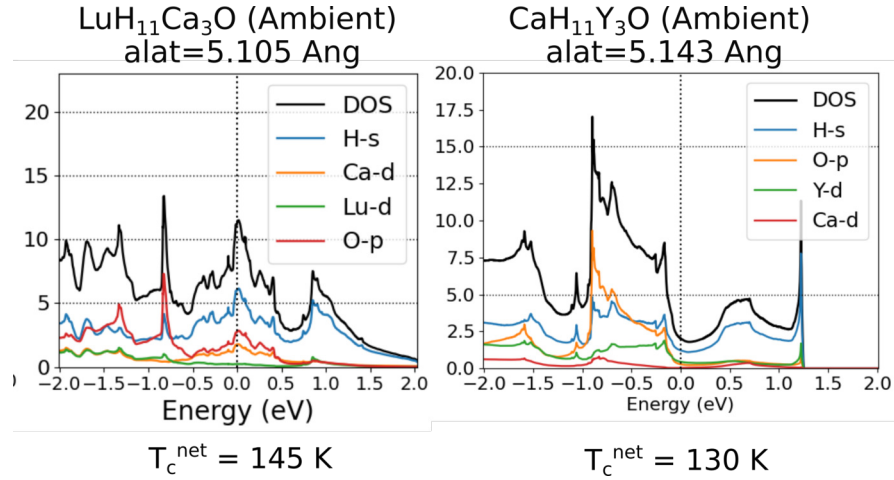

FIG. 6: PDOS and  $T_c^{\text{net}}$  of two more examples of using the structural formula. (a)  $\text{LuH}_{11}\text{Ca}_3\text{N}$ , (b)  $\text{CaH}_{11}\text{Y}_3\text{O}$ .

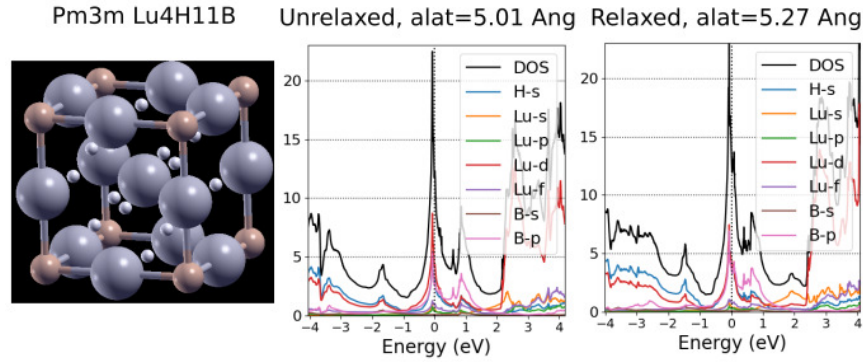

FIG. 7: PDOS of  $\text{Lu}_4\text{H}_{11}\text{B}$  with DFT+U,  $U=7.5$  eV. There is a flat band at  $E_F$  of hybridized character which persists upon relaxation of the unit cell.

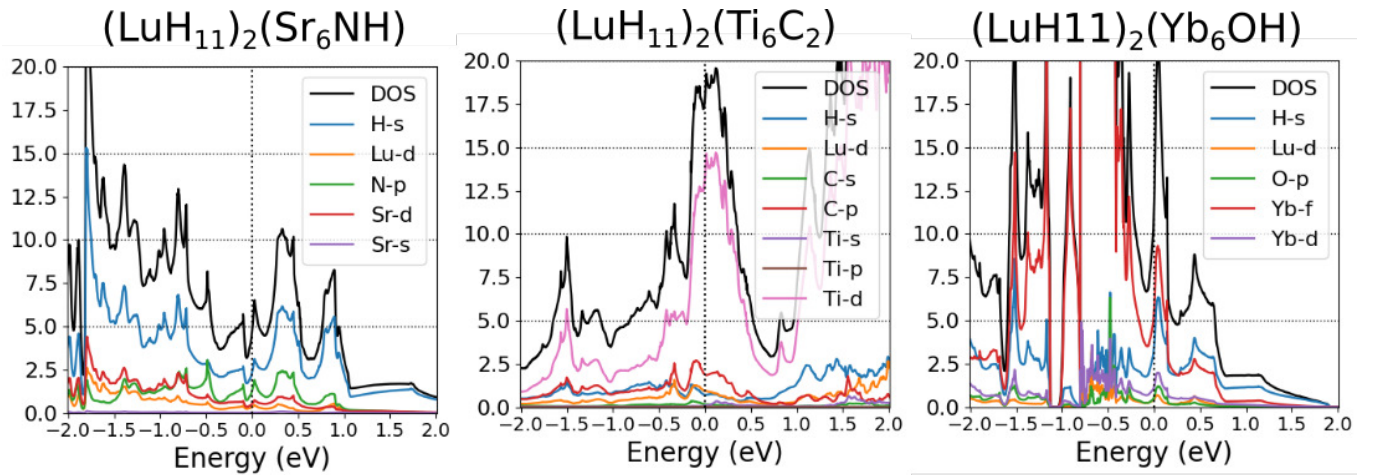

FIG. 8: PDOS calculated for three examples using  $R=\text{Lu}$ . One uses  $X=\text{Sr}$ ,  $Y=\text{N}$ ,  $Z=\text{H}$  (left), another uses  $X=\text{Ti}$ ,  $Y=Z=\text{C}$  (middle), and the last uses  $X=\text{Yb}$ ,  $Y=\text{O}$ ,  $Z=\text{H}$  (right).

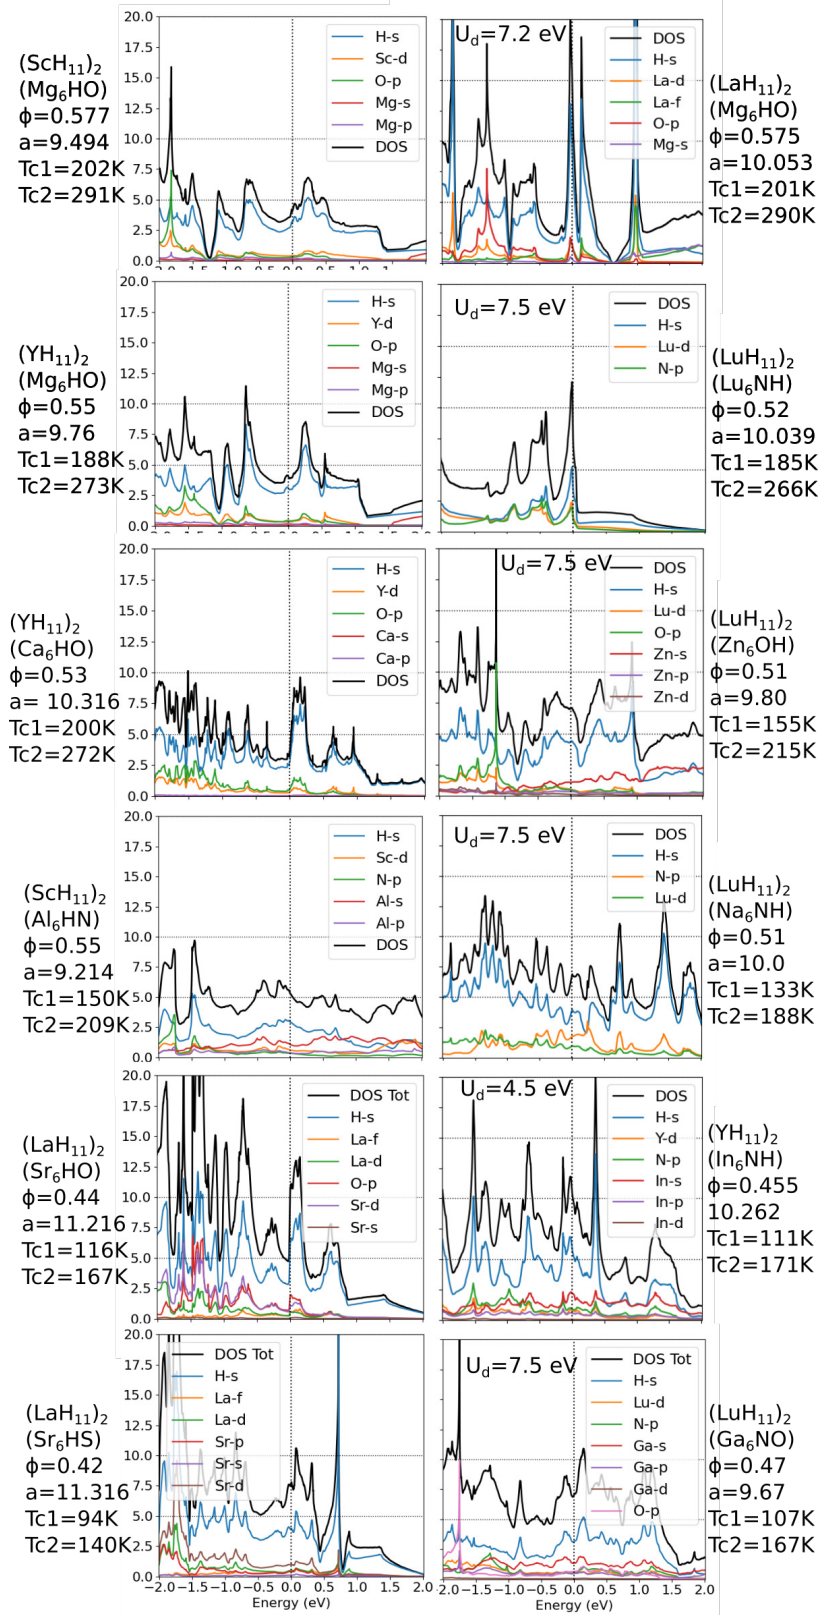

FIG. 9: The PDOS calculated for twelve quaternary hydride compositions using the formula discussed in the text. For each, the lattice constant, computed  $\phi_{iso}^{net}$ , and estimated  $T_c$ s are listed. Both columns are ordered from highest estimated  $T_c$  (top) to lowest (bottom). For structures in the left column +U was not applied, and the structures in the right column had the indicated  $U$ -value applied for the R atoms. All structures were relaxed using PBE from the high-symmetry starting point defined by the structure formula.

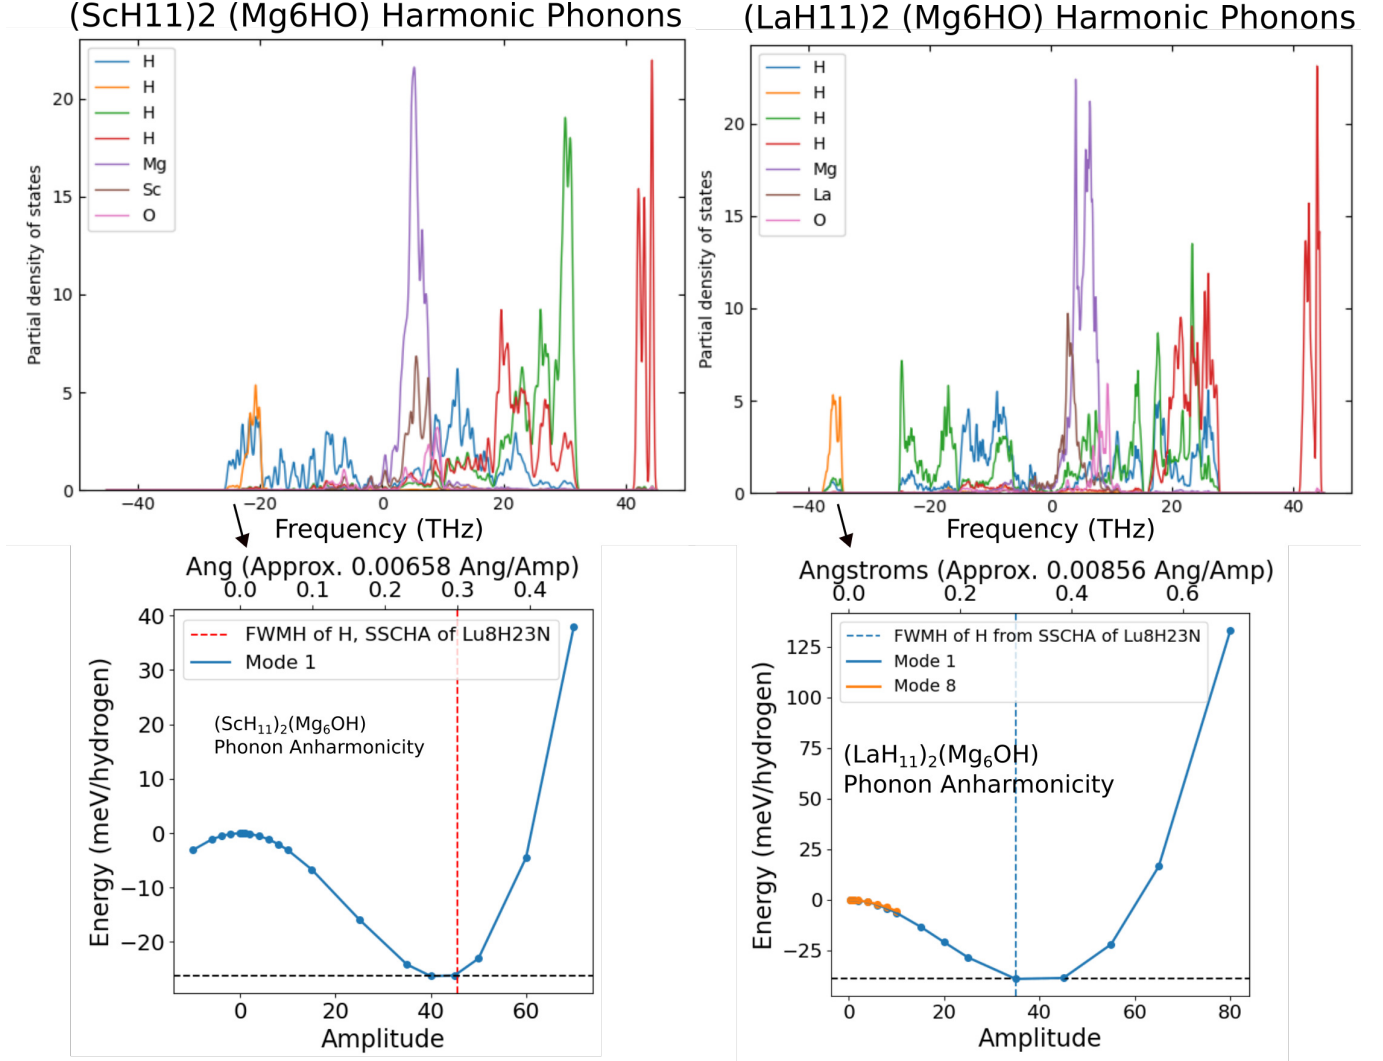

FIG. 10: Top: Atom-resolved phonon density of states (pdDOS) in ambient conditions for  $(\text{RH}_{11})_2(\text{Mg}_6\text{OH})$  for  $\text{R}=\text{Sc}/\text{La}$ . There are four unique hydrogen atoms which we do not distinguish further for simplicity's sake, but both octahedral and tetrahedral hydrogen participate in the unstable modes below 0 frequency. The simple acoustic sum rule (ASR) was used. Bottom: Collective-mode reaction-coordinate DFT analysis of the  $([\text{La}/\text{Sc}]\text{H}_{11})_2(\text{Mg}_6\text{OH})$  phonon mode with largest imaginary phonon frequency. The amplitude of modulation is also translated to approximate Angstroms moved per H atom by averaging H displacements. The full-width half-maximum (FWHM) is plotted from previous work on  $\text{Lu}_8\text{H}_{23}\text{N}$  (Å) [To be submitted] indicating the amount of quantum zero point motion of a typical hydrogen.

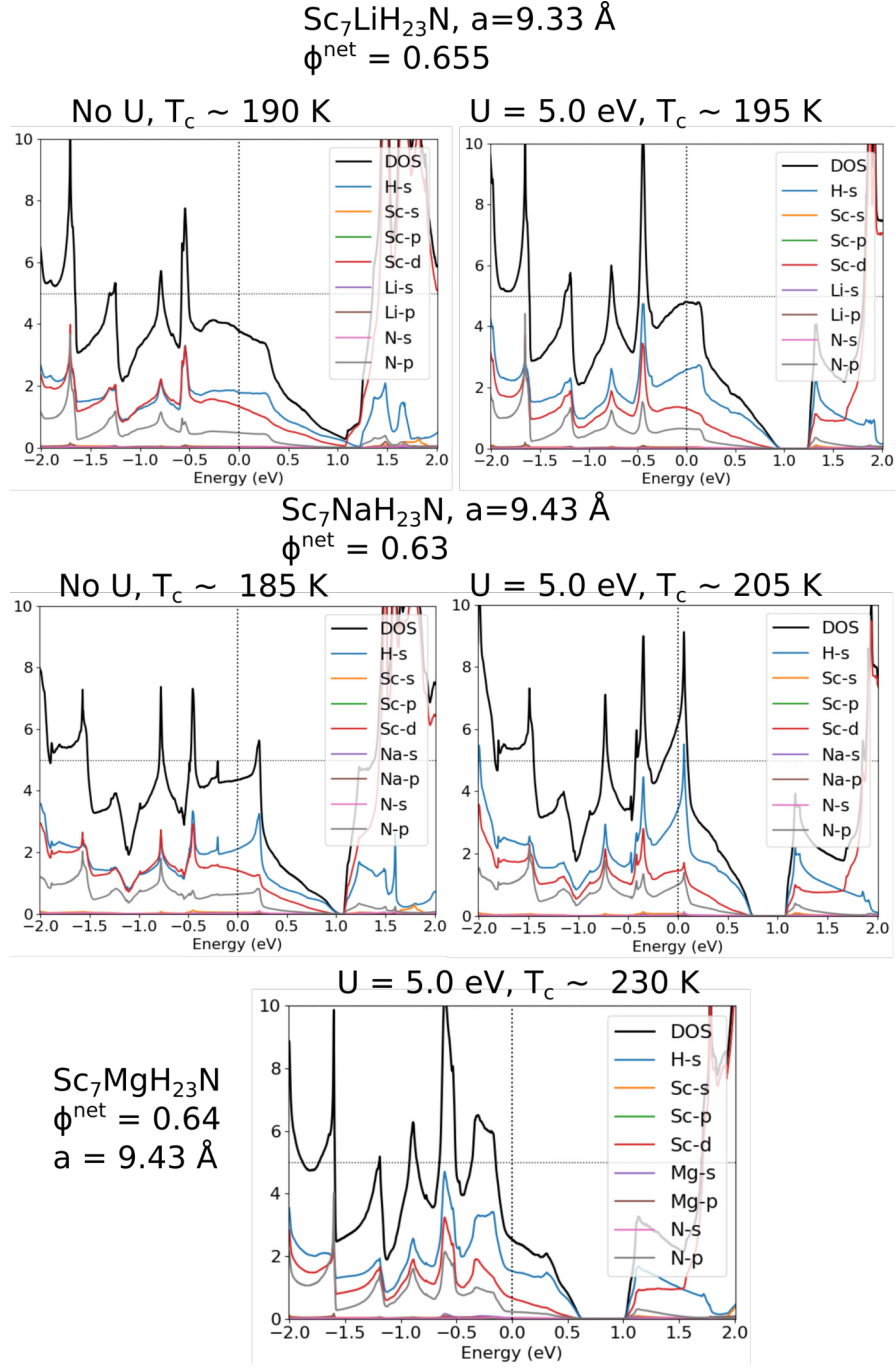

FIG. 11: PDOS,  $\phi_{\text{iso}}^{\text{net}}$  and  $T_c$  estimates of  $\text{Sc}_7\text{LiH}_{23}\text{N}$  and  $\text{Sc}_7\text{NaH}_{23}\text{N}$  with and without  $U_{\text{Sc-d}} = 5.0 \text{ eV}$ , and of  $\text{Sc}_7\text{MgH}_{23}\text{N}$  with  $U$ .

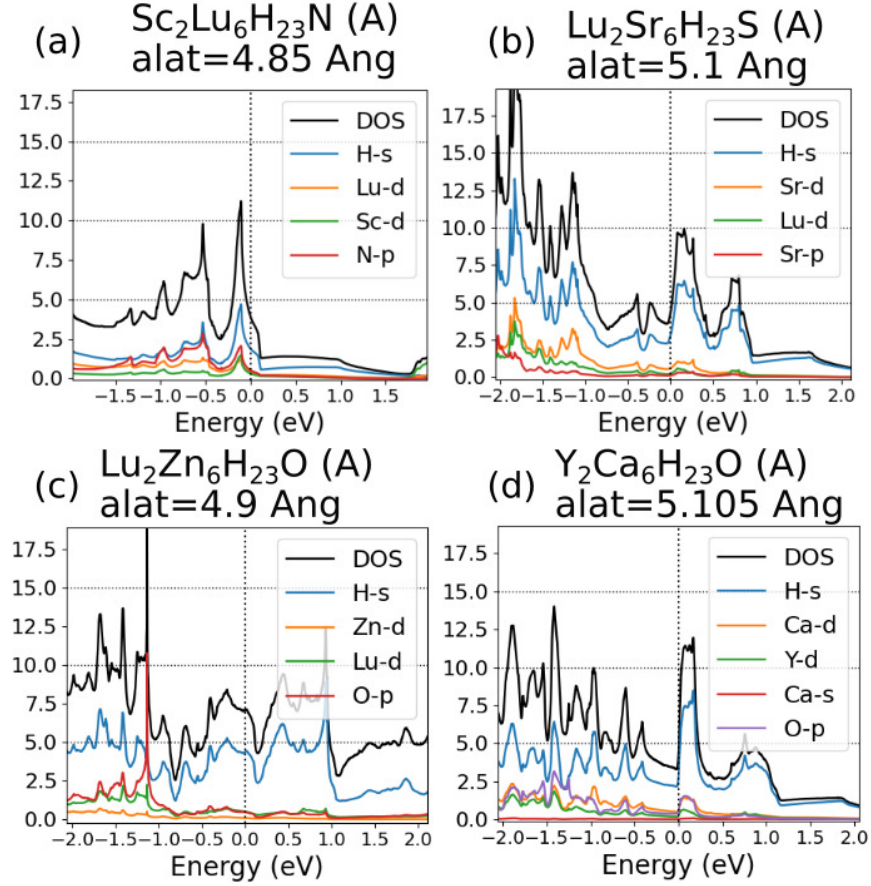

FIG. 12: The PDOS calculated for (a)  $(\text{ScH}_{11})_2(\text{Lu}_6\text{NH})$  with alat 4.85Å, (b)  $(\text{LuH}_{11})_2(\text{Sr}_6\text{HS})$  with alat 5.1Å, (c)  $(\text{LuH}_{11})_2(\text{Zn}_6\text{HO})$  with alat 4.9Å, and (d)  $(\text{YH}_{11})_2(\text{Ca}_6\text{OH})$  with alat 5.18Å

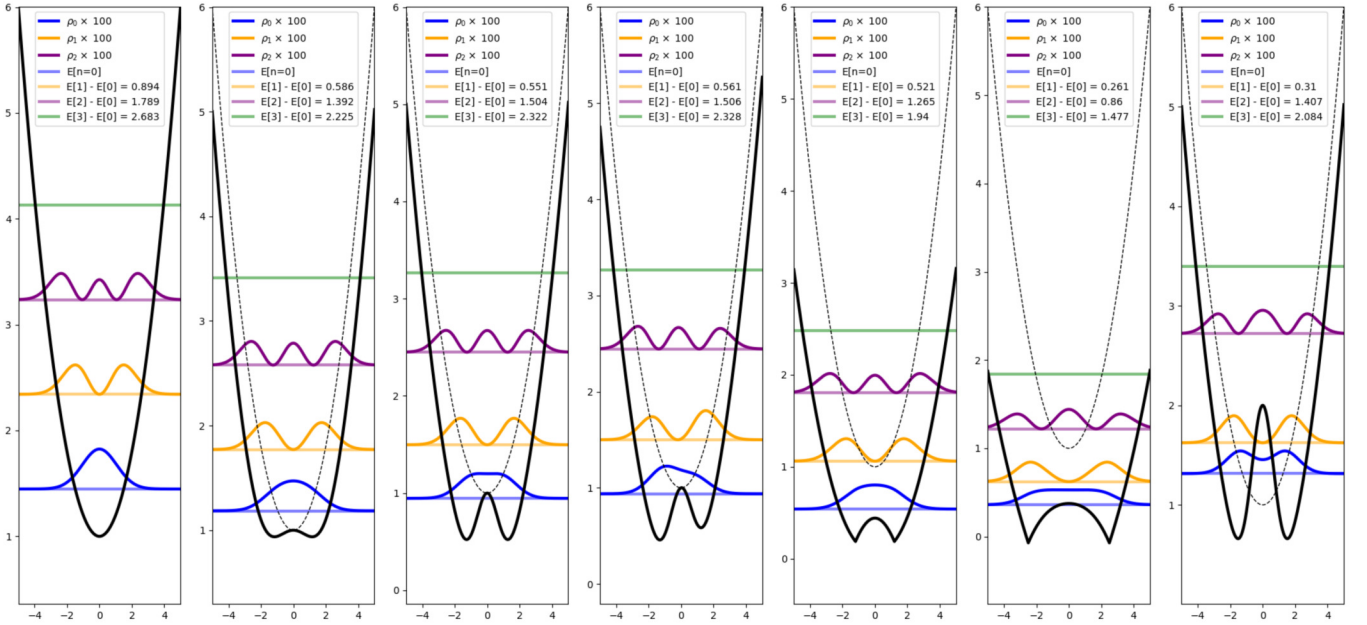

FIG. 13: Computed ground state (ground) and excited state densities (yellow, purple) for a variety of anharmonic potentials in the 1D Schrodinger equations.

## 20 GPa PDOS, undistorted structure

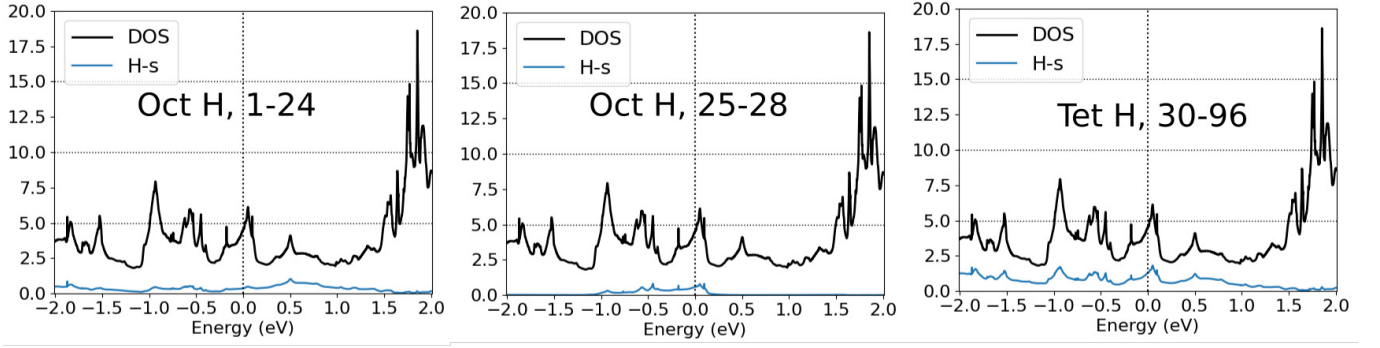

## 20 GPa PDOS, distorted structure

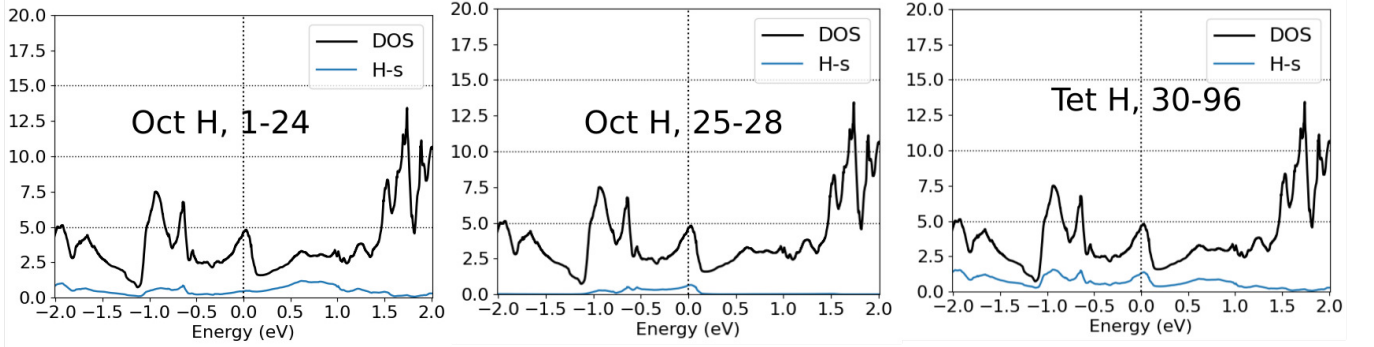

FIG. 14: PDOS of  $(\text{CaH}_{11})\text{Sc}_6\text{NH}$  resolved into the unique types of hydrogen in the system. The 24d-hydrogen, 4b hydrogen, and tetrahedral hydrogen all contribute nontrivially to  $\text{DOS}(E_F)$ , before and after the structural distortion (see main text).

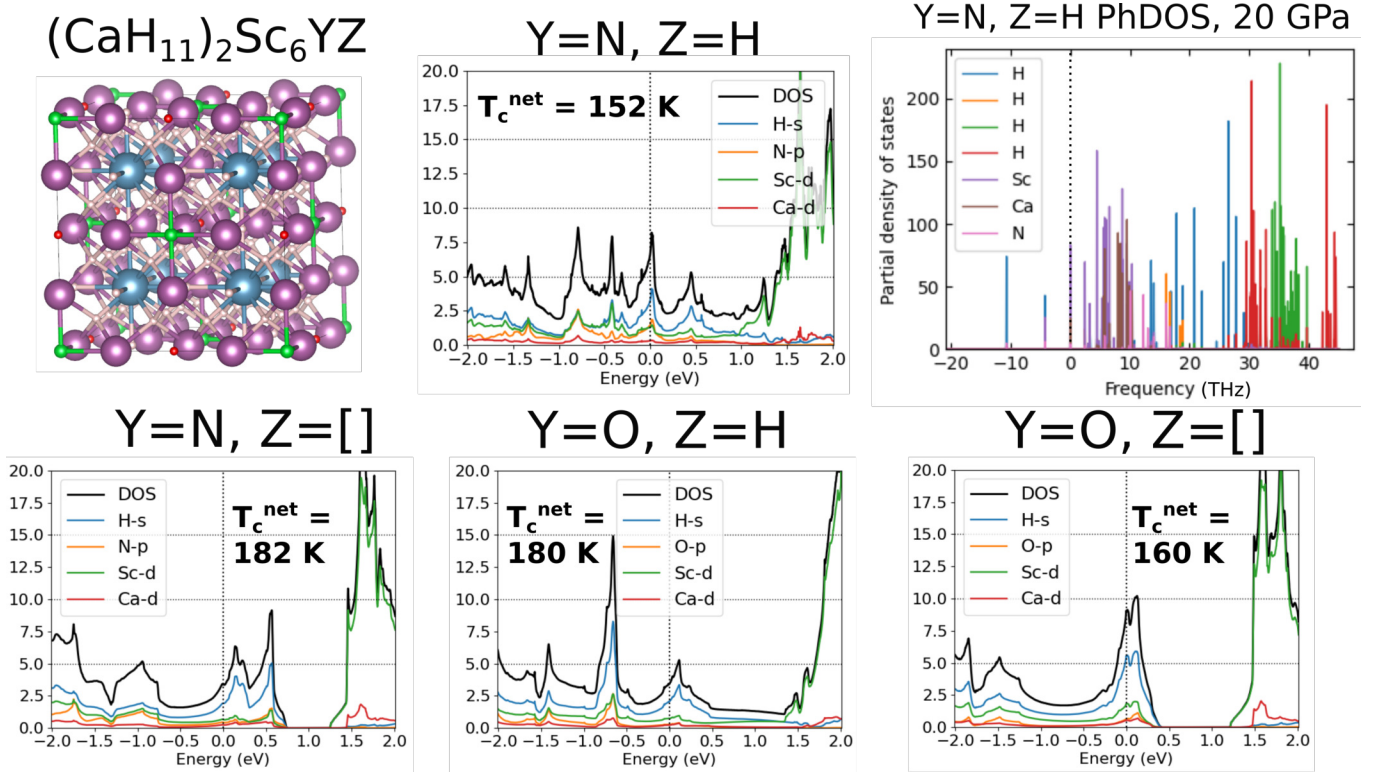

FIG. 15: PDOS of  $(\text{CaH}_{11})\text{Sc}_6\text{YZ}$  for various Y,Z, and their associated  $T_c^{\text{net}}$

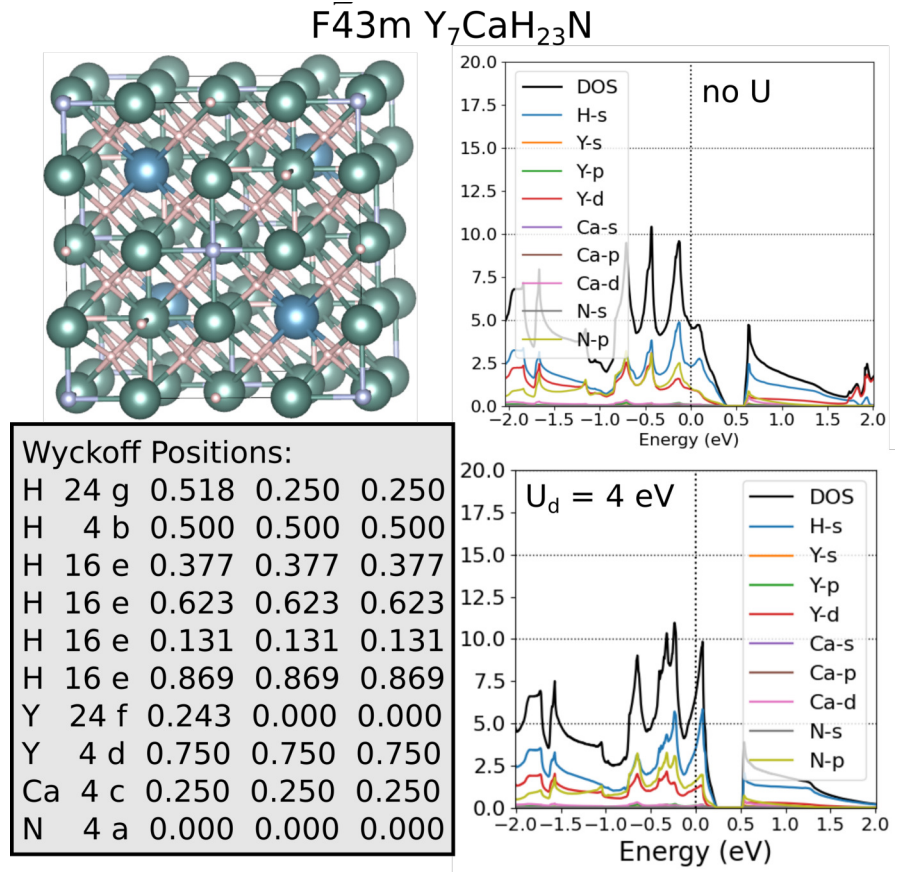

FIG. 16: Structure and PDOS of  $(YCaH_{22})(Y_6NH)$  without and with  $U = 4$  eV, and lattice constant  $10.244 \text{ \AA}$ . The  $\phi_{iso}^{net}$  increases to 0.56 due to the 24g-H compressing toward the 4d-Y upon Ca doping. The networking-value  $T_c^{net}$  we obtain using the Quantum Espresso projections is 180 K.

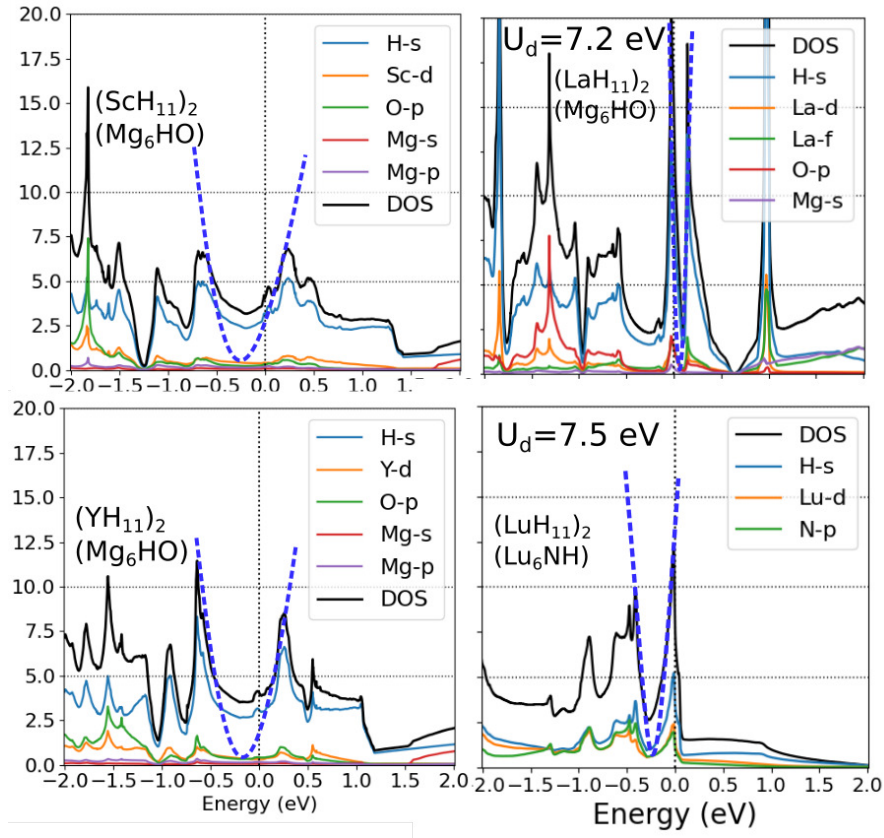

FIG. 17: PDOS of four examples following the second model structure  $(\text{RH}_{11})_2\text{X}_6\text{YZ}$  with the common U-shaped DOS near  $E_F$  highlighted.

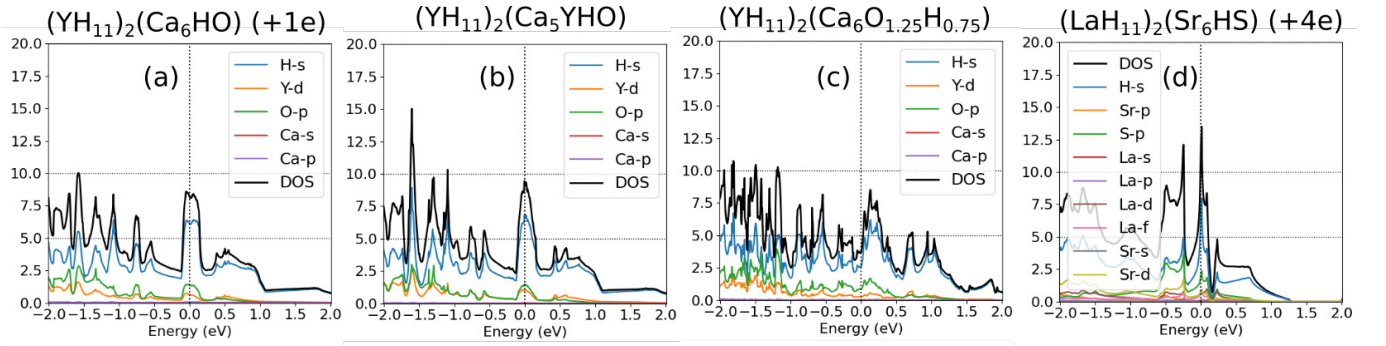

FIG. 18: PDOS calculated for doped variants of two example compositions shown in Fig. 9. Relaxation with dopants was not performed. (a)  $(\text{YH}_{11})_2(\text{Ca}_6\text{OH})$  with an extra electron added to the 32-atom primitive cell with compensating uniform background charge. (b)  $(\text{YH}_{11})_2(\text{Ca}_5\text{YOH})$  (choosing  $\text{X}'=\text{Y}$ ). (c)  $(\text{YH}_{11})_2(\text{Ca}_6\text{O}_{1.25}\text{H}_{0.75})$  (choosing  $\text{Z}'=\text{O}$ ). (d)  $(\text{LaH}_{11})_2(\text{Sr}_6\text{SH})$  with four extra electrons added to the 32-atom primitive cell.

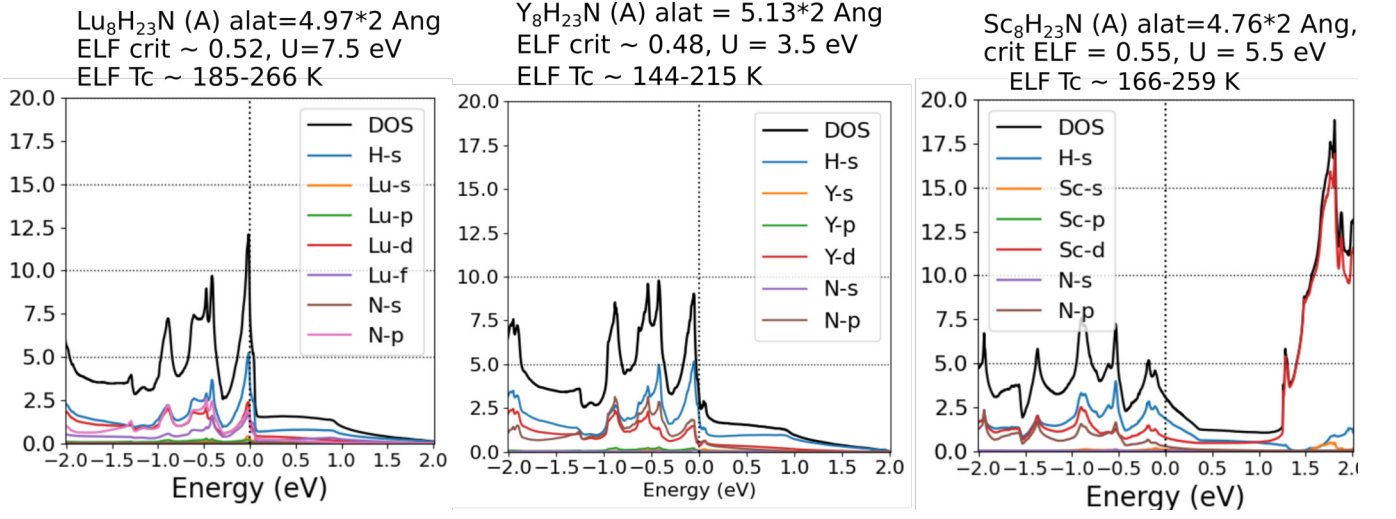

FIG. 19: PDOS of  $(\text{RH}_{11})_2(\text{R}_6\text{NH})$  using the parent structure

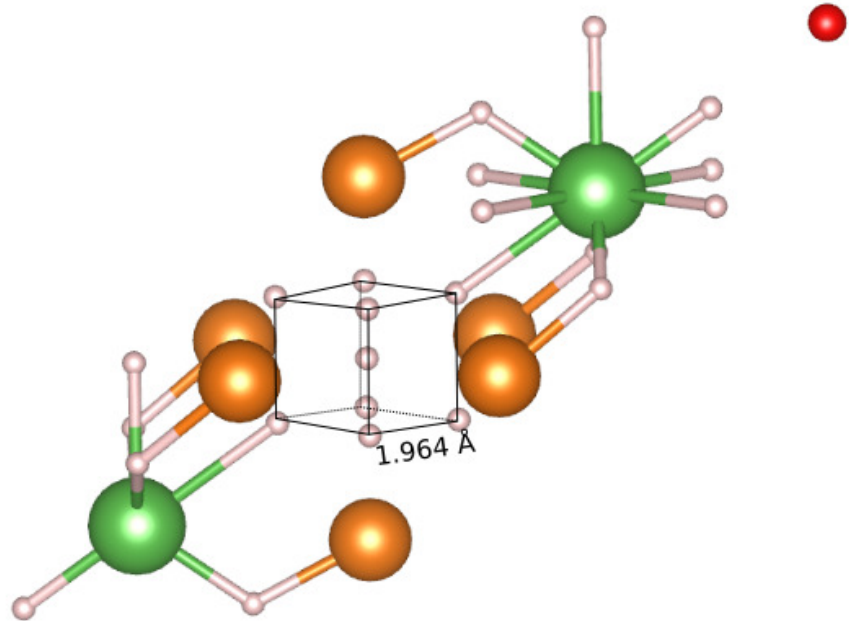

FIG. 20: Primitive cell of  $(\text{LaH}_{11})_2(\text{Mg}_6\text{OH})$  with an inner hydrogen cage visualized.

## $R_6YZ$ Charge-Donating Pocket

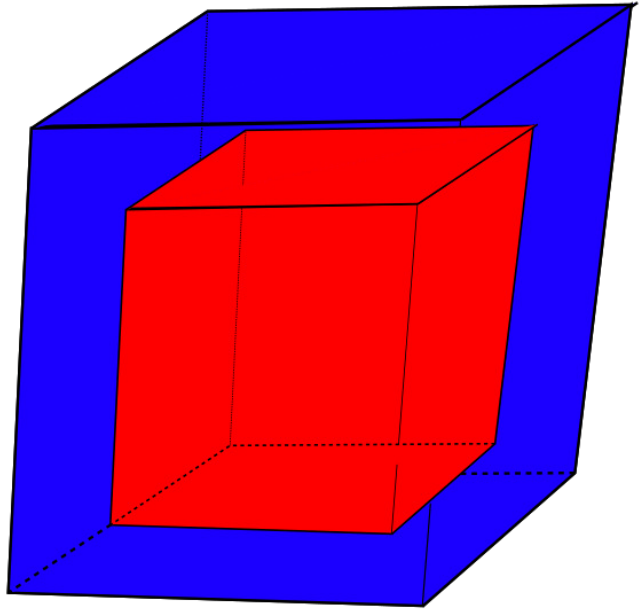

$XH_{11}$  Surroundings

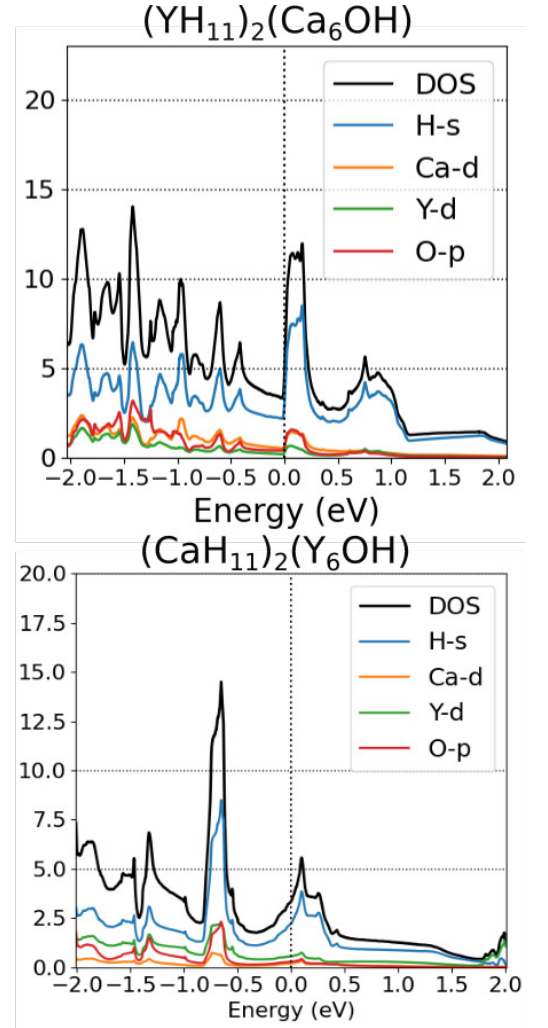

FIG. 21: We picture inverting the role of the R and X atoms (left) since the interface chemistry should be similar. Indeed, our example (right) shows that  $(YH_{11})_2(Ca_6OH)$  (lattice constant 5.158 Å) and the swapped X,R role version  $(CaH_{11})_2(Y_6OH)$  (lattice constant 5.119 Å) have a very similar DOS near  $E_F$ , with the extra electrons simply providing a hole-doping effect.

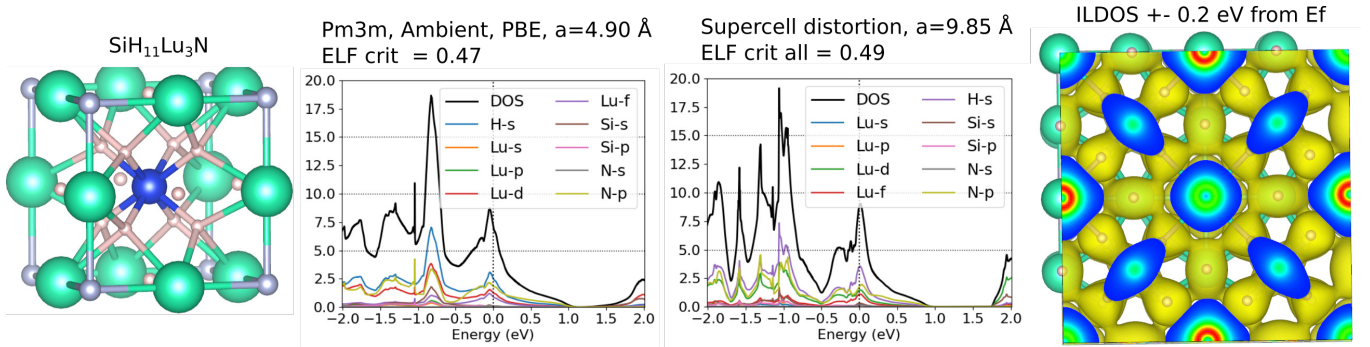

FIG. 22: We visualize  $Pm\bar{3}m$   $SiH_{11}Lu_3N$  and its PDOS, with estimated  $T_c^{net} = 90$  K. However, we found a  $2 \times 2 \times 2$  supercell relaxes the tetrahedral hydrogen sublattice saving 2.4 meV/atom and increasing the hydrogen connectivity of the lattice, resulting in  $T_c^{net} = 125$  K. The resulting PDOS is also shown, and the electron density from states near  $E_F$  is illustrated on the right.

- [1] C. Wang, S. Yi, and J.-H. Cho, Multiband nature of room-temperature superconductivity in  $\text{LaH}_{10}$  at high pressure, *Phys. Rev. B* **101**, 104506 (2020).
- [2] N. P. Salke, A. C. Mark, M. Ahart, and R. J. Hemley, Evidence for near ambient superconductivity in the  $\text{Lu-NH}$  system, arXiv preprint arXiv:2306.06301 (2023).
- [3] V. E. Antonov, V. K. Fedotov, A. S. Ivanov, A. I. Kolesnikov, M. A. Kuzovnikov, M. Tkacz, and V. A. Yartys, Lattice dynamics of high-pressure hydrides studied by inelastic neutron scattering, *J. Alloys Compd.* **905**, 164208 (2022).
- [4] R. A. Klein, R. Balderas-Xicohtencatl, J. P. Maehlen, T. J. Udovic, C. M. Brown, R. Delaplane, Y. Cheng, R. V. Denys, A. J. Ramirez-Cuesta, and V. A. Yartys, Neutron vibrational spectroscopic evidence for short H-H contacts in the  $\text{RNiInH}_{1.4;1.6}$  ( $R = \text{Ce, La}$ ) metal hydride, *J. Alloys and Compounds* **894**, 162381 (2022).
- [5] A. Denchfield, F. Belli, E. Zurek, H. Park, and R. J. Hemley, Quantum stabilization and flat hydrogen-based bands of nitrogen-doped lutetium hydride, arXiv preprint arXiv:2403.01350 (2024).
- [6] M. Topsakal and R. Wentzcovitch, Accurate projected augmented wave (PAW) datasets for rare-earth elements ( $\text{RE} = \text{La-Lu}$ ), *Computational Materials Science* **95**, 263 (2014).
- [7] T. Yamamoto, K. Kaminaga, D. Saito, D. Oka, and T. Fukumura, High electron mobility with significant spin-orbit coupling in rock-salt  $\text{YbO}$  epitaxial thin film, *Appl. Phys. Lett.* **114** (2019).
- [8] R. Koshoji, M. Fukuda, M. Kawamura, and T. Ozaki, Prediction of quaternary hydrides based on densest ternary sphere packings, *Phys. Rev. Mater.* **6**, 114802 (2022).
- [9] P. P. Ferreira, L. J. Conway, A. Cucciari, S. Di Cataldo, F. Giannessi, E. Kogler, L. T. Eleno, C. J. Pickard, C. Heil, and L. Boeri, Search for ambient superconductivity in the  $\text{Lu-N-H}$  system, *Nature Comm.* **14** (2023).
- [10] Y.-W. Fang, D. Dangic, and I. Errea, Assessing the feasibility of near-ambient conditions superconductivity in the  $\text{lu-nh}$  system, *Communications Materials* **5**, 61 (2024).
- [11] Z. Ouyang, M. Gao, and Z.-Y. Lu, Superconductivity at ambient pressure in hole-doped  $\text{LuH}_3$ , arXiv preprint arXiv:2306.13981 (2023).
- [12] R. Kataoka, T. Kimura, N. Takeichi, and A. Kamegawa, Stabilization of face-centered cubic high-pressure phase of  $\text{REH}_3$  ( $\text{RE} = \text{Y, Gd, Dy}$ ) at ambient pressure by alkali or alkaline-earth substitution, *Inorganic Chemistry* **57**, 4686 (2018).
- [13] W. Kalisvaart, R. Niessen, and P. Notten, Electrochemical hydrogen storage in  $\text{MgSc}$  alloys: A comparative study between thin films and bulk materials, *J. Alloys Compd.* **417**, 280 (2006).
- [14] L. Ouyang, F. Qin, and M. Zhu, The hydrogen storage behavior of  $\text{Mg}_3\text{La}$  and  $\text{Mg}_3\text{LaNi}_{0.1}$ , *Scripta materialia* **55**, 1075 (2006).
- [15] L. Monacelli, R. Bianco, M. Cherubini, M. Calandra, I. Errea, and F. Mauri, The stochastic self-consistent harmonic approximation: calculating vibrational properties of materials with full quantum and anharmonic effects, *J. Phys.: Condens. Matter* **33**, 363001 (2021).
- [16] C. Boonchot, P. Tsuppayakorn-Aek, U. Pinsook, and T. Bovornratanaraks, Stability and electronic structure of magnesium hydride and magnesium deuteride under high pressure, in *J. Physics: Conference Series*, Vol. 2145 (IOP Publishing, 2021) p. 012026.
- [17] A. Peles and C. G. Van de Walle, Role of charged defects and impurities in kinetics of hydrogen storage materials: A first-principles study, *Phys. Rev. B* **76**, 214101 (2007).
- [18] M. S. Salman, C. Prathana, Q. Lai, T. Wang, N. Rambhujun, K. Srivastava, and K.-F. Aguey-Zinsou, Catalysis in solid hydrogen storage: Recent advances, challenges, and perspectives, *Energy Technology* **10**, 2200433 (2022).
- [19] A. Gross and M. Scheffler, Role of zero-point effects in catalytic reactions involving hydrogen, *J. Vacuum Science & Technology A: Vacuum, Surfaces, and Films* **15**, 1624 (1997).
- [20] A. Togo, First-principles phonon calculations with phonopy and phono3py, *J. Physical Society of Japan* **92**, 012001 (2023).
- [21] R. Lucrezi, E. Kogler, S. Di Cataldo, M. Aichhorn, L. Boeri, and C. Heil, Quantum lattice dynamics and their importance in ternary superhydride clathrates, *Comm. Physics* **6**, 298 (2023).
- [22] R. Lucrezi, P. P. Ferreira, M. Aichhorn, and C. Heil, Temperature and quantum anharmonic lattice effects on stability and superconductivity in lutetium trihydride, *Nature Comm.* **15**, 441 (2024).
- [23] P. Giannozzi, O. Andreussi, T. Brumme, O. Bunau, M. B. Nardelli, M. Calandra, R. Car, C. Cavazzoni, D. Ceresoli, M. Cococcioni, *et al.*, Advanced capabilities for materials modelling with quantum espresso, *J. Physics: Cond. Matter* **29**, 465901 (2017).
- [24] G. Prandini, A. Marrazzo, I. E. Castelli, N. Mounet, and N. Marzari, Precision and efficiency in solid-state pseudopotential calculations, *npj Comp. Mater.* **4**, 1 (2018).
- [25] A. Dal Corso, Pseudopotentials periodic table: From H to Pu, *Comp. Mater. Sci.* **95**, 337 (2014).
- [26] M. Schlipf, M. Betzinger, C. Friedrich, M. Ležaić, and S. Blügel, Hse hybrid functional within the flapw method and its application to gdn, *Phys. Rev. B* **84**, 125142 (2011).
- [27] M. Kawamura, Y. Gohda, and S. Tsuneyuki, Improved tetrahedron method for the brillouin-zone integration applicable to response functions, *Phys. Rev. B* **89**, 094515 (2014).
- [28] K. Momma and F. Izumi, Vesta 3 for three-dimensional visualization of crystal, volumetric and morphology data, *J. Appl. Crystallography* **44**, 1272 (2011).
- [29] D. Chakraborty, K. Berland, and T. Thonhauser, Next-generation nonlocal van der waals density functional, *J. Chem. Theory and Comput.* **16**, 5893 (2020).
- [30] F. Belli, T. Novoa, J. Contreras-Garcia, and I. Errea, Strong correlation between electronic bonding network and critical temperature in hydrogen-based superconductors, *Nature Comm.* **12**, 5381 (2021).
- [31] J. P. Perdew, K. Burke, and M. Ernzerhof, Generalized gradient approximation made simple, *Phys. Rev. Lett.* **77**, 3865 (1996).
